# Supplementary material for: Search Improves Label for Active Learning
Source: arXiv:1602.07265 source file (2016-10-24)
Supplement: Supplementary file 1 [file appendix-agnostic.tex]

%\section{Performance Guarantees of \alga}
\section{Performance Guarantees of \textsc{A-Larch}}
\label{sec:agnostic-proof}

In this section, we present and analyze a generalization of \alga,
which is shown below as Algorithm~\ref{alg:realizableagnostic}.
In place of the upper bound $\nu$ on the error rate of $h^*$, it takes
as input an oracle $\gamma$, which takes as input a version space $V$
and returns the error rate of the optimal hypothesis $h^*$ restricted
to $\DIS(V)$:
\begin{equation}
  \Pr_{(x,y) \sim D}[ h^*(x) \neq y ,\, x \in \DIS(V) ]
  \ \leq \
  \gamma(V)
  \ \leq \
  \nu
  \quad\text{for all version spaces $V$}
  \,.
  \label{eq:gamma}
\end{equation}
Here, $\nu$ is an upper bound that must hold for all version spaces
$V$.
$\alga$ is a special case of Algorithm~\ref{alg:realizableagnostic}
where we use an oracle that always returns $\nu$, an upper bound on
the error rate of $h^*$:
\[
  \gamma(V) \ \equiv \ \nu
  \ \geq \
  \err(h^*)
  \,.
\]
This is always a valid upper bound by the law of total probability.

\paragraph{Remark.}
In many common settings, it is possible to obtain a tighter bound than
$\nu$ on the error rate of the optimal classifier in the disagreement
region.
For example, with random classification noise with noise rate $\eta$,
where the label $y$ for any given $x$ is generated by flipping the
label $h^*(x)$ with probability $\eta$, we have
\[
  \Pr_{(x,y) \sim D}[ h^*(x) \neq y ,\, x \in \DIS(V) ]
  \ = \
  \eta \cdot \Pr_{x \in D_\calX}(x \in \DIS(V))
  \,.
\]
The probability $\Pr_{x \in D_\calX}(x \in \DIS(V))$ can be
estimated very accurately just with unlabeled examples.
If we are also provided with an upper bound $\bar\eta$ on the noise
rate $\eta$, then we can use
\[
  \gamma_{\bar\eta}(V)
  \ := \
  \bar\eta \cdot \Pr_{x \in D_\calX}[x \in \DIS(V)]
\]
as the oracle $\gamma$.
Using such a tighter bound, we can prove a smaller final error rate
bound.

\begin{algorithm}[t]
\caption{Generalized \alga}
\begin{algorithmic}[1]
\REQUIRE
  Nested hypothesis classes $H_0 \subset H_1 \subset H_2 \subset \ldots$;
  oracles $\LABEL$ \& $\SEARCH$;
  oracle $\gamma$ satisfying~\eqref{eq:gamma};
  %error thresholds $\cbr{\gamma_i^k}_{i,k=0}^{\infty}$;
  learning parameter $\epsilon, \delta \in (0,1)$.
\ENSURE $\hat{h}$, a classifier with error at most $2\nu + \epsilon$.
%\STATE $L \gets $ Draw a dataset of size $\tilde{O}(\frac{\nu + \epsilon}{\epsilon^2})$ from $D_{\calX}$, query $\LABEL$ for their labels.
\STATE Initialize $k \gets 0$, $S \gets \emptyset$.
\LOOP
    \STATE Set $\delta_k = \delta/(k^2+k)$.
%    \STATE $(V_k, h_k) \gets \AL(H_k(S), \LABEL, \cbr{\gamma_i^k}_{i=0}^\infty, \epsilon, \delta_k)$
    \STATE $(V_k, h_k) \gets \AL(H_k(S), \LABEL, \gamma, \epsilon, \delta_k)$
    
    \IF{$V_k = \emptyset$}
        \STATE $k \gets k + 1$
    \ELSE 
        \STATE $e \gets \SEARCH_{H_k}(V_k)$
        
        \IF[no counterexample found]{$e = \bot$}
			\RETURN $h_k$
		\ELSE[counterexample found] 
			\STATE $S \gets S \cup \{e\}$
			\STATE $k \gets \min\{k' > k: H_{k'}(S) \neq \emptyset\}$
		\ENDIF
	\ENDIF
\ENDLOOP
\end{algorithmic}
\label{alg:realizableagnostic}
\end{algorithm}

%Denote by $V_{i,k}$ the version space in iteration $i$ when Algorithm~\ref{alg:realizableagnostic} is working with hypothesis class $H_k$. If indeed the $\gamma_i^k = \Pr(h^*(x) \neq y, x \in \DIS(V_{i,k}))$ for all $i$,$k$, then we have the following stronger error guarantee.
%
\begin{theorem}\label{thm:errorboundnu}
  Assume there is a minimal index $k^*$ and classifier $h^* =
  h_{k^*}^*$ in $H_{k^*}$ such that $\err(h^*)$ is at most $\nu$.
  If Algorithm~\ref{alg:realizableagnostic} is run with inputs hypothesis
  classes $\cbr{H_k}_{k=0}^{\infty}$, oracles $\SEARCH$ and $\LABEL$,
  oracle $\gamma$ satisfying~\eqref{eq:gamma},
%  error thresholds $\cbr{\gamma_i^k}_{i,k=0}^{\infty}$ such that for
%  all $i$,$k$ $\gamma_i^k = \Pr[h^*(x) \neq y, x \in \DIS(V_{i,k})]$,
  and learning parameters $\epsilon,\delta$ then with probability
  $1-\delta$ the returned hypothesis $\hat{h}$ satisfies
  \[
    \err(\hat{h})
    \ \leq \
%    \nu + \epsilon \,. 
    \Pr_{(x,y) \sim D}[
      h^*(x) \neq y ,\, x \notin \DIS(V_{k_0})
    ]
    + \gamma(V_{k_0}) + \epsilon
  \]
  where $k_0$ is the final value of the index $k$.
\end{theorem}

An immediate consequence of Theorem~\ref{thm:errorboundnu} is that,
if oracle $\gamma$ always returns the exact error of $h^*$ in $\DIS(V)$,
i.e. 
$\gamma(V) = \Pr_{(x,y) \sim D}[h^*(x) \neq y, x \in \DIS(V)]$,
then the error of the returned hypothesis $\hat{h}$ is at most 
$\nu + \epsilon$.

Theorem~\ref{thm:errorbound2nu} is the same as
Theorem~\ref{thm:errorboundnu}, except specialized to \alga and with
the error rate bound is $\err(\hat h) \leq 2\nu+\epsilon$.

\begin{theorem}[Query Complexity]\label{thm:querycomplexity}
  Assume there is a minimal index $k^*$ and classifier $h^* =
  h_{k^*}^*$ in $H_{k^*}$ such that $\err(h^*)$ is at most $\nu$.
  If Algorithm~\ref{alg:realizableagnostic} is run with inputs hypothesis
  classes $\cbr{H_k}_{k=0}^{\infty}$, oracles $\SEARCH$ and $\LABEL$,
  oracle $\gamma$ satisfying~\eqref{eq:gamma},
%  error thresholds $\cbr{\gamma_i^k}_{i,k=0}^{\infty}$ such that for
%  all $i$,$k$ $\gamma_i^k = \Pr[h^*(x) \neq y, x \in \DIS(V_{i,k})]$,
  and learning parameters $\epsilon,\delta$, and the disagreement
  coefficient of $H_k(S)$ at iteration $k$ is at most
  $\theta_k(\cdot)$, then, with probability $1-\delta$:
  \begin{enumerate}
    \item[(1)]
      The number of queries to oracle $\SEARCH$ is at most $k^*$.\\
    \item[(2)]
      The number of queries to oracle $\LABEL$ is at most 
      \[
        \tilde{O}\del[4]{
          k^* \cdot \max_{k \leq k^*} \theta_k(2\nu + 2\epsilon) \cdot
          d_{k^*}\left(\log \frac{1}{\epsilon}\right)^2 \cdot \del[3]{
            1 + \frac{\nu^2}{\epsilon^2}
          }
        }
      \]
  \end{enumerate}
%Assume there is a minimal index $k^*$ and classifier $h^* = h_{k^*}^*$ in $H_{k^*}$, such that $\err(h^*)$ is at most $\nu$. If Algorithm~\ref{alg:realizableagnostic} is run with inputs hypothesis classes $\cbr{H_k}_{k=0}^{\infty}$, oracles $\SEARCH$ and $\LABEL$, error thresholds $\cbr{\gamma_i^k}_{i,k=0}^{\infty}$ such that $\Pr[h^*(x) \neq y, x \in \DIS(V_{i,k})] \leq \gamma_i^k$, learning parameters $\epsilon,\delta$, and the disagreement coefficient of $H_k(S)$ at iteration $k$ is at most $\theta_k(\cdot)$, then, with probability $1-\delta$:\\
%(1) The number of queries to oracle $\SEARCH$ is at most $k^*$.\\
%(2) The number of queries to oracle $\LABEL$ is at most 
%\[ \tilde{O}(k^* \cdot \max_{k \leq k^*} \theta_k(2\nu + 2\epsilon) \cdot d_{k^*} \cdot (1 + \frac{\nu^2}{\epsilon^2})) \]
\end{theorem}

Now we prove Theorems~\ref{thm:errorbound2nu},
\ref{thm:querycomplexity2nu}, \ref{thm:errorboundnu} and
\ref{thm:querycomplexity}.
First we define some notations.
For each iteration $k$, let $E_k$ be the event in which:
\begin{quote}
  \AL succeeds with input hypothesis set $H := H_k(S)$, oracle \LABEL,
  oracle $\gamma$ satisfying~\eqref{eq:gamma}, and parameters
  $\epsilon,\delta/(k^2+k)$.
\end{quote}
%\begin{eqnarray*} 
%E_k &=&\{ \text{ $\AL$ succeeds with inputs hypothesis set $H = H_k(S)$, oracle $\LABEL$, } \\
%&& \text{\quad error threshold $\cbr{\gamma_i^k}_{i=0}^\infty$, accuracy $\epsilon$, failure probability $\delta_k$.} \}
%\end{eqnarray*}
Also define $E := \bigcap_{k \geq 0} E_k$. 
\begin{fact}
  $\P(E) \geq 1 - \delta$.
\end{fact}
\begin{proof}
  This follows from Lemma~\ref{lem:mainal} and a union bound.
\end{proof}

\begin{proof}[Proof of Theorem~\ref{thm:errorboundnu}]
  By Lemma~\ref{lem:inv}, Algorithm~\ref{alg:realizableagnostic} returns.
  Recall that $k_0$ is the round at which
  Algorithm~\ref{alg:realizableagnostic} returns. 
  Suppose $\AL(H_{k_0}(S), \LABEL, \gamma, \epsilon, \delta_{k_0})$
  halts at iteration $I_0$. 
  Then by Item 1 of Lemma~\ref{lem:mainal},
  \[
    \Pr_{(x,y) \sim D}[\hat h_{k_0}(x) \neq y,\, x \in \DIS(V_{k_0})]
    \ \leq \
    \gamma(V_{k_0}) + \epsilon
    \,.
  \]
  On the other hand, since $\SEARCH$ returns $\bot$, we have that
  $\hat h_k$ agrees with $h^*$ on the set $\calX \setminus
  \DIS(V_{k_0})$, hence
  \[
    \Pr_{(x,y) \sim D}[\hat h_{k_0}(x) \neq y,\, x \notin \DIS(V_{k_0})]
    \ = \ \Pr_{(x,y) \sim D}[h^*(x) \neq y,\, x \notin \DIS(V_{k_0})]
    \,.
  \]
  The claim now follows by the law of total probability.
\end{proof}

\begin{proof}[Proof of Theorem~\ref{thm:errorbound2nu}]
  Recall that $\alga$ is a special case of
  Algorithm~\ref{alg:realizableagnostic} where $\gamma(V) \equiv \nu$
  for all version spaces $V$.
  We have
  \[
    \Pr_{(x,y) \sim D}[h^*(x) \neq y,\, x \notin \DIS(V_{k_0})]
    \ \leq \
    \Pr_{(x,y) \sim D}[h^*(x) \neq y]
    \ = \ \err(h^*) \ \leq \ \nu
    \,.
  \]
  Therefore the bound from Theorem~\ref{thm:errorboundnu} becomes
  \[
    \err(\hat h)
    \ \leq \
    \Pr_{(x,y) \sim D}[
      h^*(x) \neq y ,\, x \notin \DIS(V_{k_0})
    ]
    + \gamma(V_{k_0}) + \epsilon
    \ \leq \
    2\nu + \epsilon
    \,.
    \qedhere
  \]
%
%
%
%By Lemma~\ref{lem:inv}, Algorithm~\ref{alg:realizableagnostic} returns.
%Denote by $k_0$ the round at which Algorithm~\ref{alg:realizableagnostic} returns. 
%
%Suppose $\AL(H_{k_0}(S), \LABEL, \cbr{\gamma_i^k}_{i=0}^\infty, \epsilon, \delta_{k_0})$ halts at iteration $I_0$. 
%Then by item 1 of Lemma~\ref{lem:mainal}, and $\gamma_{I_0-1}^{k_0} = \nu$, we get that
%\[ \Pr[\hat h_{k_0}(x) \neq y, x \in \DIS(V_{k_0})] \leq \nu + \epsilon \]
%On the other hand, since $\SEARCH$ returns $\bot$, we have that $\hat h_{k_0}$ agrees with $h^*$ on the set $\calX \setminus \DIS(V_{k_0})$, hence
%\[ \Pr[\hat h_{k_0}(x) \neq y, x \notin \DIS(V_{k_0})] = \Pr[h^*(x) \neq y, x \notin \DIS(V_{k_0})] \leq \nu \]
%We conclude that 
%\[ \Pr[\hat h(x) \neq y] = \Pr[\hat h_{k_0}(x) \neq y] \leq 2\nu + \epsilon\]
%by adding together the two sources of error.
\end{proof}

\begin{proof}[Proofs of Theorems~\ref{thm:querycomplexity} and
  Theorem~\ref{thm:querycomplexity2nu}]
  These are immediate consequences of
  Lemmas~\ref{lem:inv},~\ref{lem:qcsearch} and~\ref{lem:qclabel}
  (below).
\end{proof}

%\begin{proof}[Proof of Theorem~\ref{thm:querycomplexity2nu}]
%  Recall that $\alga$ is a special case of
%  Algorithm~\ref{alg:realizableagnostic} where $\gamma(V) \equiv \nu$
%  for all version spaces $V$.
%
%Recall that $\alga$ is a special case of Algorithm~\ref{alg:realizableagnostic} where $\gamma_i^k = \nu$ for all $i$,$k$.
%Note that $\Pr[h^*(x) \neq y, x \in \DIS(V_{i,k})] \leq \Pr[h^*(x) \neq y] = \nu$. The theorem immediately follows from Theorem~\ref{thm:querycomplexity} by setting all $\gamma_i^k$'s to be $\nu$.
%\end{proof}
%
\subsection{Auxiliary Lemmas}

\begin{lemma}
On event $E$, Algorithm~\ref{alg:realizableagnostic} returns, and maintains the invariant that $k \leq k^*$. 
\label{lem:inv}
\end{lemma}
\begin{proof}
(1) Initially, $k = 0 \leq k^*$ satisfies the invariant.

(2) Suppose at the start of the loop, $k < k^*$.  We claim that Algorithm~\ref{alg:realizableagnostic} either returns, or keeps $k \leq k^*$ at the end of the loop. By definition of $E_k$, $\AL$ succeeds, thus it returns some version space $V_k$. If $V_k$ is empty, then by line 6, $k$ gets incremented and is still at most $k^*$. Otherwise $V_k$ is nonempty. We consider $e$, the result of $\SEARCH_{H_k}(V_k)$. If $e = \bot$, then Algorithm~\ref{alg:realizableagnostic} returns at this round. If $e$ is some example $(x, h^*(x))$, then $h^*$ is consistent with the updated set $S$, thus $H_{k^*}(S) \neq \emptyset$. Therefore, the updated $k$ is at most $k^*$. 

(3) Suppose at the start of the loop, $k = k^*$, we claim that Algorithm~\ref{alg:realizableagnostic} returns at this round. Note that $h^* = h_{k^*}^*$ is the optimal hypothesis in $H_{k^*}(S)$. By definition of $E_{k^*}$, $\AL$ succeeds, thus by item 2 of Lemma~\ref{lem:mainal}, the version space $V_k$ returned is nonempty and contains $h^* = h_{k^*}^*$. Therefore $\SEARCH_{H_k}(V_k)$ returns $\bot$, and Algorithm~\ref{alg:realizableagnostic} returns at this round.
\end{proof}
\begin{lemma}[Query Complexity of $\SEARCH$]
On event $E$, the total number of queries to $\SEARCH$ is at most $k^*$.
\label{lem:qcsearch}
\end{lemma}
\begin{proof}
On event $E$, first by Lemma~\ref{lem:inv}, Algorithm~\ref{alg:realizableagnostic} maintains the invariant that $k \leq k^*$. We denote by $k_0$ the round at which Algorithm~\ref{alg:realizableagnostic} returns. Before round $k_0$ each call of $\SEARCH$ increases $k$ by at least $1$. Thus the total number of queries to $\SEARCH$ is at most $k_0$, which is at most $k^*$.
\end{proof}

%Suppose this is not the case, i.e. in some stage of Algorithm~\ref{alg:realizableagnostic}, $k$ exceeds $k^*+1$. Consider the first time this event happens, Algorithm~\ref{alg:realizableagnostic} must be executing line 10 or line 19. 
%\paragraph{Case 1:} If Algorithm~\ref{alg:realizableagnostic} is executing line 10, then $k$ before the update must be $k^*$. Thus,
%\[ \err(\hat{h}_m,T_m) > \nu + \sqrt{\nu \skmdm} + \skmdm \]
%But we know that on event $E$, when working with $H_{k^*}(S)$,
%\[ \err(\hat{h}_m,T_m) \leq \nu + \sqrt{\nu \skmdm} + \skmdm\]
%Thus we get a contradiction.
%\paragraph{Case 2:} If Algorithm~\ref{alg:realizableagnostic} is executing line 19, then line 17 means that $k < k^*$. We also know that $h_{k^*}^*$ is in $H_{k^*}(S)$, therefore $k$ should be updated to $k^*$, contradiction.
%Next, notice that each time $\SEARCH$ is queried, $k$ gets incremented by 1. We conclude that the number of queries to $\SEARCH$ is at most $

\begin{lemma}[Query Complexity of $\LABEL$]
On event $E$, the total number of queries to $\LABEL$ is at most
$\tilde{O}(k^* \cdot \max_{k \leq k^*} \theta_k(2\nu + 2\epsilon) \cdot d_{k^*}(\log \frac{1}{\epsilon})^2 \cdot (1 + \frac{\nu^2}{\epsilon^2}) )$.
\label{lem:qclabel}
\end{lemma}
\begin{proof}
On event $E$, by Lemma~\ref{lem:inv},
Algorithm~\ref{alg:realizableagnostic} maintains the invariant that $k
\leq k^*$. For each iteration $k$, by definition of $E_k$ and
Lemma~\ref{lem:mainal}, the number of queries to $\LABEL$ is at most
$\tilde{O}(\theta_k(2\nu + 2\epsilon) \cdot d_k (\log \frac{1}{\epsilon})^2 \cdot (1 +
\frac{\nu^2}{\epsilon^2}))$. Therefore the total number of queries to
$\LABEL$ is at most $\tilde{O}(k^* \cdot \max_{k \leq k^*}
\theta_k(2\nu + 2\epsilon) \cdot d_{k^*}(\log \frac{1}{\epsilon})^2 \cdot (1 + \frac{\nu^2}{\epsilon^2}) )$.
\end{proof}
