# Supplementary material for: Search Improves Label for Active Learning
Source: arXiv:1602.07265 source file (2016-10-24)
Supplement: Supplementary file 2 [file appendix-al.tex]

\section{Active Learning Algorithm \textsc{AL}}
\label{sec:mainal}

In this section, we present an agnostic active learning algorithm $\AL$ in Algorithm~\ref{alg:realizableagnostic}. $\AL$ works when the model may be ``misspecified", i.e. $h^*$ may not be in hypothesis class $H$. This brings additional challenges to the design active learning algorithms since typical active learning only aims at finding a low error hypothesis within a fixed hypothesis class $H$.  We want $\AL$ to return (with low query complexity of $\LABEL$), if and only if one of the following two events happen:
\begin{enumerate}
\item The error of the best hypothesis in $H$ is too large. In this case we are confident that $h^*$ is not in $H$.
\item We have found a good enough hypothesis. In this case, we additionally return a version space $V$ to pass the subsequent $\SEARCH$ test.
\end{enumerate}
Unlike traditional active learning algorithms, $\AL$ has an additional input oracle $\gamma$ that returns upper bounds on error of $h^*$ in the disagreement regions. 

Lemma~\ref{lem:mainal} shows that when $\AL$ is working with $H_{k^*}$, $h^*$ is always kept in the version space. Otherwise, when $\AL$ is working with $H_k$ for some $k < k^*$, it may halt early(line 14) by testing if the error of the optimal hypothesis in $H_k$ in the disagreement region $V_{i-1}$ is greater than $\gamma_{i-1}$. In this case, $\AL$ returns an empty version space.
Finally, in line 17, $\AL$ checks that the excess error of the returned hypothesis $\hat{h}_i$ inside the disagreement region is at most $\gamma_{i-1} + \epsilon$. If the condition is satisfied, $\AL$ halts and returns version space $V_{i-1}$ and hypothesis $\hat{h}_i$.
%If the condition is satisfied, and the resulting version space $V$ passes the test of $\SEARCH$ oracle (i.e. $\SEARCH(V)$ returns $\bot$), then $\hat{h}$ is guaranteed to have excess error at most $\epsilon$.

\begin{algorithm}
  \caption{$\AL$}
  \label{alg:mainal}
  \begin{algorithmic}[1]
    \REQUIRE Hypothesis set $H$; oracle $\LABEL$; oracle $\gamma$ satisfying~\eqref{eq:gamma};
    learning parameters $\epsilon,\delta \in (0,1)$

    \ENSURE Version space $V$ and hypothesis $\hat{h}$.
    
    \STATE Initialize $V_0 \gets H$

    \FOR{$i = 1, 2, \dotsc$}
      \STATE $S_i \gets \emptyset$

      \FOR{$j = 1, 2, \dotsc, 2^i$}
        \STATE $x_{i,j} \gets \text{independent draw from $D_\calX$}$
        (the corresponding label is hidden)

        \IF{$x_{i,j} \in \DIS(V_{i-1})$}

          \STATE $S_i \gets S_i \cup \cbr[0]{ (x_{i,j},\LABEL(x_{i,j})) }$

        \ELSE
        
          \STATE $S_i \gets S_i \cup \cbr[0]{ (x_{i,j},V_{i-1}(x_{i,j})) }$

        \ENDIF

      \ENDFOR
      
      \STATE $\hat{h}_i \gets \arg\min\cbr{\err(h, S_i): h \in V_{i-1}}$

      \STATE $\gamma_{i-1} \gets \gamma(V_{i-1})$
      
      \STATE Update version space: \[ V_i \gets \cbr{h \in V_{i-1}: \Pr_{(x,y) \sim S_i}[h(x) \neq y] \leq \Pr_{(x,y) \sim S_i}[\hat{h}_i(x) \neq y] + 3\sqrt{\Pr_{(x,y) \sim S_i}[\hat{h}_i(x) \neq y]\sigma(2^i, \delta_i)} + 4\sigma(2^i, \delta_i) } \]

      \IF{$\Pr_{(x,y) \sim S_i}[\hat{h}_i(x) \neq y] > \gamma_{i-1} + \sqrt{\gamma_{i-1}\sigma(2^i, \delta_i)} + \sigma(2^i, \delta_i)$}
%[Or $\Pr_{S_i}(\hat{h}_i(x) \neq y) > \nu + \sqrt{\nu\sigma(2^i, \delta_i)} + \sigma(2^i, \delta_i)$]
      \RETURN $(\emptyset, \hat{h}_i)$ 

      \ENDIF

      \IF{$\Pr_{(x,y) \sim S_i}[\hat{h}_i(x) \neq y] + \sqrt{\Pr_{(x,y) \sim S_i}[\hat{h}_i(x) \neq y] \sigma(2^i, \delta_i)} + \sigma(2^i, \delta_i) \leq \gamma_{i-1} + \epsilon$}

        \RETURN $(V_{i-1}, \hat{h}_i)$

      \ENDIF

    \ENDFOR

  \end{algorithmic}
\end{algorithm}

\subsection{Performance Guarantees of \textsc{AL}}
%Recall that the optimal hypothesis $h^*$ may not necessarily be in $H$.

\begin{lemma}[Guarantees of Algorithm $\AL$] 
Suppose algorithm $\AL$ is run with inputs hypothesis class $H$ with VC dimension $d < \infty$, oracle $\LABEL$, oracle $\gamma$ satisfying Equation~\eqref{eq:gamma}, accuracy $\epsilon$, and failure probability $\delta$. 
Additionally, the disagreement coefficient of $H$ with respect to $D_\calX$ is $\theta(\cdot)$
%, and suppose there is a hypothesis $h^*$ ($h^*$ is not necessarily in $H$) such that $\err(h^*) = \nu$,
Then with probability $1-\delta$, if $\AL$ returns at iteration $I$, then the following hold:
\begin{enumerate}
\item If the final version space $V$ returned is nonempty, then $\hat{h}$ and $V$ is such that
\[ \P[\hat{h}(x) \neq y, x \in \DIS(V)] - \gamma(V) \leq \epsilon \]

\item Denote by $h^*_H$ the optimal hypothesis in $H$, i.e. $h^*_H := \arg\min\cbr{\err(h): h \in H}$. If $h^*_H = h^*$ almost surely, then the returned version space $V$ is nonempty and contains $h^*_H$.

\item The total number of calls to the oracle $\LABEL$ is at most 
\[ \tilde{O} \del{ \theta(2\nu + 2\epsilon) \cdot d \left(\log\frac{1}{\epsilon}\right)^2 \cdot \left(1 + \frac{\nu^2}{\epsilon^2}\right) } \]
\end{enumerate}
\label{lem:mainal}
\end{lemma}

When the $(1-\delta)$-probability event in Lemma~\ref{lem:mainal} happens, we say that $\AL$ succeeds.

\begin{proof}[Proof of Lemma~\ref{lem:mainal}]
Note that the version spaces are nested, i.e. $V_0 \supseteq V_1 \supseteq \dotsb$, hence
$\DIS(V_0) \supseteq \DIS(V_1) \supseteq \dotsb$ as well. Observe that $S_i$ is an iid sample of size $2^i$ from a
distribution (call it $D_{i-1}$) over labeled examples $(x,y)$, where
$x \sim D_\calX$ and the conditional distribution of $y$ given $x$ is
\[
  D_{i-1}(y|x) \ := \
  \begin{cases}
    \mathbf{1}\{y = V_{i-1}(x)\} & \text{if $x \notin \DIS(V_{i-1})$} \,, \\
    D(y|x) & \text{if $x \in \DIS(V_{i-1})$} \,,
  \end{cases}
\]
where $\mathbf{1}\{\Phi\} = 1$ if $\Phi$ is true, and 
$\mathbf{1}\{\Phi\} = 0$ if $\Phi$ is false.
%Recall that $I$ is the iteration when $\AL$ returns.

Let $E_i$ be the event in which the following hold:
\begin{enumerate}
  \item
    Every $h \in V_i$ satisfies
    \[
      \Pr_{(x,y) \sim D_{i-1}}
      [ h(x) \neq y ]
      \ \leq \ 
      \Pr_{(x,y) \sim S_i}[h(x) \neq y]
      +
      \sqrt{ \Pr_{(x,y) \sim S_i}[h(x) \neq y]
      \sigma(2^i,\delta_i)}
      +
      \sigma(2^i,\delta_i)
      \,.
    \]
    \[
    \Pr_{(x,y) \sim S_i}
    [ h(x) \neq y ]
    \ \leq \ 
    \Pr_{(x,y) \sim D_{i-1}}[h(x) \neq y]
    +
    \sqrt{ \Pr_{(x,y) \sim D_{i-1}}[h(x) \neq y]
    \sigma(2^i,\delta_i)}
    +
    \sigma(2^i,\delta_i)
    \,.
    \]

  \item The number of $\LABEL$ queries at iteration $i$ is at most
    \[
      2^i \Pr_{x \sim D_\calX}[x \in \DIS(V_{i-1})] + O\del{
        \sqrt{2^i \Pr_{x \sim D_\calX}[x \in \DIS(V_{i-1})] \log(1/\delta_i)} + \log(1/\delta_i)
      }
      \,,
    \]
\end{enumerate}

Using the VC inequality and Lemma~\ref{lem:invbern}, along with the union bound, $\Pr(E_i) \geq 1 - \delta_i$. 
Define $E: =\cap_{i=1}^{\infty} E_i$, by union bound, $\Pr(E) \geq 1 - \delta$.
Suppose $E$ happens.

1. Recall that $\AL$ ends at iteration $I$. If $V$ returned is nonempty, then line 18 is satisfied at iteration $I$. 
Note that the error of the returned classifier $\hat{h}_I$ on $D_{I-1}$ can be written as
\begin{eqnarray*} 
\Pr_{(x,y) \sim D_{I-1}}[ \hat{h}_I(x) \neq y ] &=& \Pr_{(x,y) \sim D}[ \hat{h}_I(x) \neq y, x \in \DIS(V_{I-1})] + \Pr_{(x,y) \sim D}[ \hat{h}_i(x) \neq V_{I-1}(x), x \notin \DIS(V_{I-1})]\\
&=& \Pr_{(x,y) \sim D_{I-1}}[ \hat{h}_I(x) \neq y, x \in \DIS(V_{I-1})]
\end{eqnarray*}

Then, by definition of $E_I$,
$\hat{h}_I$ is such that
    \[
      \Pr_{(x,y) \sim D_{I-1}}
      [ \hat{h}_I(x) \neq y ]
      \ \leq \ 
      \Pr_{(x,y) \sim S_I}[\hat{h}_I(x) \neq y]
      +
      \sqrt{ \Pr_{(x,y) \sim S_I}[\hat{h}_I(x) \neq y]
      \sigma(2^I,\delta_I)}
      +
      \sigma(2^I,\delta_I)
      \,
      \leq \gamma_{I-1} + \epsilon
    \]
That is,
\[ \Pr[\hat{h}_I(x) \neq y, x \in \DIS(V_{I-1})] - \gamma_{I-1} \leq \epsilon \]
Since the $V$ returned is $V_{I-1}$ and the $\hat{h}$ returned is $\hat{h}_I$, we get,
\[ \Pr[\hat{h}(x) \neq y, x \in \DIS(V)] - \gamma(V) \leq  \epsilon \]

2. 
First we show by induction that $h^*_H$ is in $V_i$ for all $i$. 
\item \paragraph{Base Case.} For $i = 0$, the fact follows trivially since $V_0 = H$.
\item \paragraph{Inductive Case.} Suppose $h^*_H$ is in $V_{i-1}$. It can be easily seen that $h^*$ is the optimal hypothesis under distribution $D_{i-1}$. Therefore, $\Pr_{(x,y) \sim D_{i-1}}[h^*(x) \neq y] \leq \Pr_{(x,y) \sim D_{i-1}}[\hat{h}_i(x) \neq y]$.
Now, by definition of $E_1$,
\begin{eqnarray*}  
    \Pr_{(x,y) \sim S_i}
    [ h^*_H(x) \neq y ]
    \ &\leq& \ 
    \Pr_{(x,y) \sim D_{i-1}}[h^*_H(x) \neq y]
    +
    \sqrt{ \Pr_{(x,y) \sim D_{i-1}}[h^*_H(x) \neq y] \sigma(2^i,\delta_i)}
    +
    \sigma(2^i,\delta_i) \\
    \ &\leq& \ 
    \Pr_{(x,y) \sim D_{i-1}}[\hat{h}_i(x) \neq y]
    +
    \sqrt{ \Pr_{(x,y) \sim D_{i-1}}[\hat{h}_i(x) \neq y]
    \sigma(2^i,\delta_i)}
    +
    \sigma(2^i,\delta_i) \\
    \ &\leq& \ 
    \Pr_{(x,y) \sim S_i}[\hat{h}_i(x) \neq y]
    +
    3\sqrt{ \Pr_{(x,y) \sim S_i}[\hat{h}_i(x) \neq y]
    \sigma(2^i,\delta_i)}
    +
    4\sigma(2^i,\delta_i)
\end{eqnarray*}
Therefore, by definition of $V_i$, $h^*_H$ is in $V_i$. This completes the induction.

Now suppose $h^*_H = h^*$ almost surely. We show that the condition in line 14 is never satisfied. To see this, note that for each $i$, since $h^*_H$ is in $V_{i-1}$, $\Pr_{(x,y) \sim S_i}[\hat{h}_i(x) \neq y] \leq \Pr_{(x,y) \sim S_i}[h^*_H(x) \neq y]$.
Thus, by definition of $E_1$,
\begin{eqnarray*}
\Pr_{(x,y) \sim S_i}[\hat{h}_i(x) \neq y] &\leq& \Pr_{(x,y) \sim S_i}[h^*_H(x) \neq y] \\
&\leq& \Pr_{(x,y) \sim D_{i-1}}[h^*_H(x) \neq y] + \sqrt{\Pr_{(x,y) \sim D_{i-1}}[h^*_H(x) \neq y]\sigma(2^i,\delta_i)} + \sigma(2^i,\delta_i)\\
&=& \Pr_{(x,y) \sim D_{i-1}}[h^*(x) \neq y] + \sqrt{\Pr_{(x,y) \sim D_{i-1}}[h^*(x) \neq y]\sigma(2^i,\delta_i)} + \sigma(2^i,\delta_i)\\
&\leq& \gamma_{i-1} + \sqrt{\gamma_{i-1}\sigma(2^i,\delta_i)} + \sigma(2^i,\delta_i)
\end{eqnarray*}
where the last inequality uses the fact that by Equation~\eqref{eq:gamma}, $\Pr_{(x,y) \sim D_{i-1}}[h^*(x) \neq y] = \Pr_{(x,y) \sim D}[h^*(x) \neq y, x \in \DIS(V_{i-1})] \leq \gamma(V_{i-1})$.
Recall that $\AL$ returns at iteration $I$, therefore it must exit through line 19, and the version space $V_{I-1}$ is nonempty, since $h^*_H \in V_{I-1}$. Thus we get the claim.

3. (1) We first show that the version space $V_i$ is always contained in a ball of small radius for those iterations in which $\AL$ does not return. Specifically we have the following claim.
\item 
\begin{claim}
If $i \leq I-1$, then for every $h, h'$ in $V_i$,
\[ \Pr_{(x,y) \sim D}[h(x) \neq h'(x)] \leq 2\gamma_{i-1} + 16\sqrt{\gamma_{i-1}\sigma(2^i,\delta_i)} + 30\sigma(2^i,\delta_i) \]
\end{claim}
\begin{proof}
If $i \leq I-1$, then neither the condition in line 14 nor the condition in line 17 is satisfied. 

First, for every $h$ in $V_i$,
\[ \Pr_{(x,y) \sim S_i}[ h(x) \neq y ] \leq \Pr_{(x,y) \sim S_i}[\hat{h}_i(x) \neq y] + 3\sqrt{\Pr_{(x,y) \sim S_i}[\hat{h}_i(x) \neq y] \sigma(2^i,\delta_i)} + 4\sigma(2^i,\delta_i) \]
and since line 14 is not satisfied, we know that
\[ \Pr_{(x,y) \sim S_i}[\hat{h}_i(x) \neq y] \leq \gamma_{i-1} + \sqrt{\gamma_{i-1}\sigma(2^i,\delta_i)} + \sigma(2^i,\delta_i) \]
Thus,
\begin{equation} 
\Pr_{(x,y) \sim S_i}[ h(x) \neq y ] \leq \gamma_{i-1} + 6\sqrt{\gamma_{i-1}\sigma(2^i,\delta_i)} + 10\sigma(2^i,\delta_i)
\label{eqn:erremph}
\end{equation}
By definition of event $E_i$, we also have
\[ \Pr_{(x,y) \sim D_{i-1}}[ h(x) \neq y ] \leq \Pr_{(x,y) \sim S_i}[ h(x) \neq y ] + \sqrt{\Pr_{(x,y) \sim S_i}[ h(x) \neq y ]\sigma(2^i,\delta_i)} + \sigma(2^i,\delta_i)\]
Hence,
\[ \Pr_{(x,y) \sim D_{i-1}}[ h(x) \neq y ] \leq \gamma_{i-1} + 8\sqrt{\gamma_{i-1}\sigma(2^i,\delta_i)} + 15\sigma(2^i,\delta_i)\]
Therefore, for any $h$, $h'$ in $V_i$, we have
\begin{eqnarray*}
\Pr_{x \sim D_\calX}[ h(x) \neq h'(x) ] &\leq& \Pr_{(x,y) \sim D_{i-1}}[ h(x) \neq y ] + \Pr_{(x,y) \sim D_{i-1}}[ h'(x) \neq y ] \\
&\leq& 2\gamma_{i-1} + 16\sqrt{\gamma_{i-1}\sigma(2^i,\delta_i)} + 30\sigma(2^i,\delta_i)
\end{eqnarray*}
The claim follows.
\end{proof}

(2) Next we bound the label complexity per iteration. First we show a property regarding the iterations in which $\AL$ does not return. 
\begin{claim}
If $i \leq I - 1$, then
\[ \gamma_{i-1} + 8\sqrt{\gamma_{i-1} \sigma(2^i, \delta_i)} + 15\sigma(2^i, \delta_i) \geq \gamma_{i-1} + \epsilon\]
\label{cla:stop}
\end{claim}
\begin{proof}
If $i \leq I - 1$, then neither the condition in line 14 nor the condition in line 17 is satisfied. Since the condition in line 17 is not satisfied, we know that
\[ \Pr_{S_i}[\hat{h}_i(x) \neq y] + \sqrt{\Pr_{S_i}[\hat{h}_i(x) \neq y] \sigma(2^i, \delta_i)} + \sigma(2^i, \delta_i) \geq \gamma_{i-1} + \epsilon\]
Also, we know that by Equation~\eqref{eqn:erremph}, 
\[ \Pr_{S_i}[\hat{h}_i(x) \neq y] \leq \gamma_{i-1} + 6\sqrt{\gamma_{i-1} \sigma(2^i, \delta_i)} + 10\sigma(2^i, \delta_i) \]
The claim follows by standard algebra.
\end{proof}

By Claim~\ref{cla:stop} and $\gamma_{i-1} = \gamma(V_{i-1}) \leq \nu$, the disagreement region $\DIS(V_i)$ is contained in $\B_{H}(\hat{h}_i, 2\nu + 16\sqrt{\nu \sigma(2^i,\delta_i)} + 30\sigma(2^i,\delta_i))$, thus its size can be bounded as
\begin{eqnarray*} 
\Pr_{x \sim D_\calX} [x \in \DIS(V_i)] &\leq& \theta(2\nu + 2\epsilon)(2\nu + 16\sqrt{\nu \sigma(2^i, \delta_i)} + 30\sigma(2^i, \delta_i)) \\
&\leq& \theta(2\nu + 2\epsilon)(10\nu + 38\sigma(2^i, \delta_i))
\end{eqnarray*}
By definition of $E_i$, the number of queries to $\LABEL$ is at most
\[ 2^i \Pr_{x \sim D_\calX}[x \in \DIS(V_{i-1})] + O\del{\sqrt{2^i \Pr_{x \sim D_\calX}[x \in \DIS(V_{i-1})] \log(1/\delta_i)} + \log(1/\delta_i)}\]
which is at most
\[ O\del{2^i \cdot \theta(2\nu + 2\epsilon) \cdot (\nu + \sigma(2^i, \delta_i)) }\]

(3) We bound $I$, the number of iterations of $\AL$. By Claim~\ref{cla:stop}, 
\[ 8\sqrt{\gamma_{I-2} \sigma(2^{I-1}, \delta_{I-1})} + 15\sigma(2^{I-1}, \delta_{I-1}) \geq \epsilon \] 
Since $\gamma_{I-2} \leq \nu$, we have that $8\sqrt{\nu \sigma(2^{I-1}, \delta_{I-1})} + 15\sigma(2^{I-1}, \delta_{I-1}) \geq \epsilon$.
Hence 
\[ 8\sqrt{\nu \sigma(2^{I-1}, \delta_{I-1})} \geq \frac{\epsilon}{2} \text{ or } 15\sigma(2^{I-1}, \delta_{I-1}) \geq \frac{\epsilon}{2} \]
we have
\[ \sigma(2^{I-1}, \delta_{I-1}) \geq \frac{\epsilon^2}{256\nu} \text{ or } \sigma(2^{I-1}, \delta_{I-1}) \geq \frac{\epsilon}{30}\]
By Fact~\ref{fact:sigma}, we get
\[ 2^I \leq O\del{ \frac{\nu}{\epsilon^2} \left(d \log\frac{\nu}{\epsilon^2} + \log\frac{1}{\delta} \right) } \text{ or } 2^I \leq O \del{ \frac{1}{\epsilon} \left(d \log\frac{1}{\epsilon} + \log\frac{1}{\delta} \right) }\]
This implies that
\[ 2^I \leq O\del{ \frac{\nu + \epsilon}{\epsilon^2} \cdot \left(d \log\frac{1}{\epsilon} + \log\frac{1}{\delta}\right)  }\]

(4) 
From the upper bound on $2^I$ in item (3), we get that 
\[ I = O \del{\log\frac{d}{\epsilon} + \log\log\frac{1}{\delta}} \]
Now, combining the results in items (2), (3), we get that the number of $\LABEL$ queries is bounded by
\begin{eqnarray*} 
&& \sum_{i=1}^I O\del{2^i \cdot \theta(2\nu + 2\epsilon) \cdot (\nu + \sigma(2^i, \delta_i))} \\
&=& O\del{\theta(2\nu + 2\epsilon) \cdot \left(\sum_{i=1}^I 2^i (\nu + \sigma(2^i, \delta_i))\right) } \\
&=& O\del{\theta(2\nu + 2\epsilon) \cdot \left(\nu 2^I + \sum_{i=1}^I 2^i \frac{d\ln(2^i) + \ln(\frac{i^2+i}{\delta})}{2^i} \right) } \\
&=& O\del{\theta(2\nu + 2\epsilon) \cdot \left(\nu 2^I + d I^2 + I \log\frac{1}{\delta} \right) }\\
&=& O\del{\theta(2\nu + 2\epsilon) \cdot \left(\frac{\nu^2 + \epsilon\nu}{\epsilon^2}(d\log\frac{1}{\epsilon} + \log\frac{1}{\delta}) + d (\log\frac{d}{\epsilon} + \log\log\frac{1}{\delta})^2 + (\log\frac{d}{\epsilon} + \log\log\frac{1}{\delta}) \log\frac{1}{\delta} \right) } \\
&=& \tilde{O}\del{\theta(2\nu + 2\epsilon) \cdot d(\log\frac{1}{\epsilon})^2 \cdot (1 + \frac{\nu^2}{\epsilon^2})}
\end{eqnarray*}
\end{proof}
%<<<<<<< HEAD
%=======
%&=& O\del{\theta(2\nu + 2\epsilon) \cdot \left(\nu 2^I + d I^2 \right) }\\
%&=& O\del{\theta(2\nu + 2\epsilon) \cdot \left(d\log\frac{1}{\epsilon} \cdot \frac{\nu^2 + \epsilon\nu}{\epsilon^2} + d \left(\log\frac{1}{\epsilon}\right)^2 + d(\log d)^2 \right) } \\
%&=& \tilde{O}\del{\theta(2\nu + 2\epsilon) \cdot d\left(\log\frac{1}{\epsilon}\right)^2 \cdot \left(1 + \frac{\nu^2}{\epsilon^2}\right)}
%>>>>>>> 31070c47305fd191e45adb945d9d8147e32fb3c5
